# Supplementary material for: Precision of Treatment Hierarchy: A Metric for Quantifying Certainty in Treatment Hierarchies from Network Meta-Analysis
Source: arXiv:2501.11596 ancillary file (2025-01-20)
Supplement: Supplementary file 1 [file POTH_SI.pdf]

# Supplementary Information

## Precision of Treatment Hierarchy: A Metric for Quantifying Certainty in Treatment Hierarchies from Network Meta-Analysis

Wigle, A.      Béliveau, A.      Salanti, G.      Rücker, G.      Schwarzer, G.      Mavridis, D.  
Nikolakopoulou, A.

### 1 Ranking Probabilities in the Minimum-Certainty Hierarchy Scenario

In Section 2.1, we defined the scenario where there is minimum certainty in a ranking to be the case when all SUCRA values are equal to 0.5. We illustrate this scenario where all ranking distributions are flat, that is, the probability that treatment  $i$  takes rank  $k$  is equal to  $1/n$  for all  $i$  and  $k$  from 1 to  $n$ . However, other configurations of ranking probabilities are possible.

In Table 1, we show two illustrative examples where the SUCRA values of all  $n = 4$  treatments are equal to 0.5, but the ranking probabilities are not all equal to  $1/n$ . In the first scenario, the ranking distribution for treatment 3 is no longer flat. The probabilities are now higher for ranks 2 and 3 and lower for ranks 1 and 4. This corresponds to a reduction in the variance of treatment 3's ranking distribution compared to the variance of a flat ranking distribution. However, the ranking distribution of treatment 4 must also now be non-flat to compensate for this and maintain all SUCRA values equal to 0.5. The ranking distribution of treatment 4 now has higher probabilities at the highest and lowest ranks, corresponding to an increase in its variance compared to a flat distribution. In general, if the variance of one treatment's ranking distribution is less than that of a flat ranking distribution, the variance of the ranking distribution of another treatment (or treatments) must be greater than that of a flat ranking distribution. Recall that in Section 2.4, we argued that the variance of a treatment's ranking distribution is a measure of the certainty in that treatment's ranking. Thus, when all SUCRAs are 0.5, any treatment with more certainty in its place in the hierarchy will be balanced by a reduction in the certainty of the place of one or more other treatments.

Scenario 2 shows another example where the ranking distribution of treatments 3 and 4 are not flat and all SUCRA values are equal to 0.5. In this case, the variance of the ranking distributions for treatments 3 and 4 are equal to the variance of a flat ranking distribution. These distributions can be described as multimodal, since each treatment has two different ranks with increased probabilities, and those ranks are not adjacent (for treatment 3, the ranks are 1 and 3). This shows that there is still very little certainty about which rank the treatments are likely to take in the hierarchy. Although the distributions are not flat, they have the same variance as a flat ranking distribution, and they provide similar information about which ranks the treatments are likely to take.

In summary, multiple configurations of probabilities are possible which give the minimum certainty in hierarchy scenario. If all distributions are not flat, any increase in certainty (reduction in variance) must be compensated by a decrease in certainty (increase in variance) in the ranking distributions of one or more treatments. Multimodality in the ranking distributions which does not change the certainty in a treatment's rank is also possible. Thus, all possible configurations of ranking probabilities where  $\text{SUCRA}(i) = 0.5$  for all  $i$  provide the same amount of certainty about the treatment hierarchy overall.

### 2 POTH with Clusters of Treatments

To exemplify POTH, consider a hypothetical network with  $n$  treatments, where there are  $m < n/2$  equally sized clusters of equivalent treatments, and  $m$  is a factor of  $n$ . For example, for  $m = 2$  and even  $n$ , we have a cluster of  $n/2$  "good" treatments and a cluster of  $n/2$  "bad" treatments. Table 2 shows the ranking probabilities for this case. The largest possible number of clusters  $m$  is  $n/2$ . In this section, we calculate POTH for this general situation.

The difference between the expected ranks in cluster  $p$  and  $l$  is equal to

$$|p - l| \frac{n}{m},$$

which means the difference in SUCRAs between treatments in clusters  $p$  and  $l$  is equal to

$$|p - l| \left( \frac{n}{m(n-1)} \right). \tag{1}$$

Table 1: Two scenarios illustrating different joint ranking distributions where all SUCRAs are equal to 0.5. In Scenario 1, the certainty in the rank of treatment 3 is increased, with an equal and opposite decrease in the certainty of the rank of treatment 4. In Scenario 2, both treatments 3 and 4 have multimodal ranking distributions which have equal certainty to those treatments with flat ranking distributions.

| Rank ( $k$ )   | Scenario 1        |      |      |      | Scenario 2        |      |      |      |
|----------------|-------------------|------|------|------|-------------------|------|------|------|
|                | Treatment ( $i$ ) |      |      |      | Treatment ( $i$ ) |      |      |      |
|                | 1                 | 2    | 3    | 4    | 1                 | 2    | 3    | 4    |
| 1              | 0.25              | 0.25 | 0.10 | 0.40 | 0.25              | 0.25 | 0.30 | 0.20 |
| 2              | 0.25              | 0.25 | 0.40 | 0.10 | 0.25              | 0.25 | 0.10 | 0.40 |
| 3              | 0.25              | 0.25 | 0.40 | 0.10 | 0.25              | 0.25 | 0.40 | 0.10 |
| 4              | 0.25              | 0.25 | 0.10 | 0.40 | 0.25              | 0.25 | 0.20 | 0.30 |
| SUCRA          | 0.5               | 0.5  | 0.5  | 0.5  | 0.5               | 0.5  | 0.5  | 0.5  |
| E(rank( $i$ )) | 2.5               | 2.5  | 2.5  | 2.5  | 2.5               | 2.5  | 2.5  | 2.5  |

Table 2: Table of ranking probabilities corresponding to the hypothetical scenario where half of the treatments perform equally well and half equally poorly (the two-group example). The values in the table correspond to  $p_{ik}$ , the probability of treatment  $i$  taking rank  $k$ .

| Rank ( $k$ ) | Treatment ( $i$ )     |          |          |                      |     |          |
|--------------|-----------------------|----------|----------|----------------------|-----|----------|
|              | 1                     | ...      | $n/2$    | $n/2 + 1$            | ... | $n$      |
| 1            | $2/n$                 | ...      | $2/n$    | 0                    | ... | 0        |
| $\vdots$     | $\vdots$              | $\ddots$ | $\vdots$ | 0                    | ... | $\vdots$ |
| $n/2$        | $2/n$                 | ...      | $2/n$    | 0                    | ... | 0        |
| $n/2 + 1$    | 0                     | ...      | 0        | $2/n$                | ... | $2/n$    |
| $\vdots$     | $\vdots$              | $\ddots$ | $\vdots$ | $2/n$                | ... | $\vdots$ |
| $n$          | 0                     | ...      | 0        | $2/n$                | ... | $2/n$    |
| SUCRA        | $(3n - 2)/(4(n - 1))$ |          |          | $(n - 2)/(4(n - 1))$ |     |          |

To calculate POTH for arbitrary  $m$ , we use the fact that the variance can be written as a sum of pairwise differences, that is, we can write

$$\begin{aligned}
S^2(n) &= \frac{1}{n} \frac{1}{2n} \sum_{i=1}^n \sum_{j=1}^n (\text{SUCRA}(i) - \text{SUCRA}(j))^2 \\
&= \frac{1}{n} \frac{1}{2n} \left(\frac{n}{m}\right)^2 \sum_{p=1}^m \sum_{l=1}^m (p - l)^2 \left(\frac{n}{m(n-1)}\right)^2 \\
&= \frac{m^2 - 1}{m^2} \frac{n^4}{12(n-1)^2}.
\end{aligned}$$

The POTH for a network with  $m$  equally-sized clusters of treatments is therefore

$$\text{POTH} = \frac{12(n-1)}{(n+1)} S^2(n) = \frac{m^2 - 1}{m^2} \frac{n^2}{n^2 - 1}. \quad (2)$$

For example, for  $m = 2$  clusters of size  $\frac{n}{2}$ , the POTH is equal to

$$\text{POTH} = \frac{3n^2}{4(n^2 - 1)}. \quad (3)$$

If we fix the number of clusters and increase the number of treatments, the value of POTH goes to  $(m^2 - 1)/m^2$ . For the case of  $m = 2$  clusters, as  $n$  approaches infinity, the POTH approaches 0.75 from above. This is because the certainty about the rankings within clusters decreases as the number of treatments in the clusters increase, but we always have certainty about the relative ranking of the two clusters.

If we fix the number of treatments  $n$  and increase the number of clusters  $m$  to its maximum value of  $n/2$ , the POTH becomes  $(n^2 - 4)/n^2$ . If we increase  $n$  and keep the maximum value of clusters, the POTH goes to 1. As  $n$  increases, the number of distinguishable hierarchy positions (clusters) increases, leading to higher certainty in the ranking.

### 3 Networks Producing Smallest and Largest POTH in NMA Database

The network which produced the smallest POTH observed in the database of NMAs investigated the risk of death for different terms of dual antiplatelet therapy after drug-eluting stents [Bulluck et al., 2015]. There were four different time periods (treatments) investigated and data were taken from seven studies. The record ID in **nmadb** is 482231.

The network which produced the largest POTH observed in the database of NMAs regarded the relative risk of major cardiovascular events at different statin doses [Ribeiro et al., 2013]. Statins were classified as low, intermediate, and high doses and compared to placebo, resulting in four treatments total. There were 39 studies in the network. The record ID in **nmadb** is 501379.

The estimated between-study variance  $\tau^2$ , the  $I^2$ , and POTH for both networks are shown in Table 3. Forest plots for both networks are shown in Figure 1.

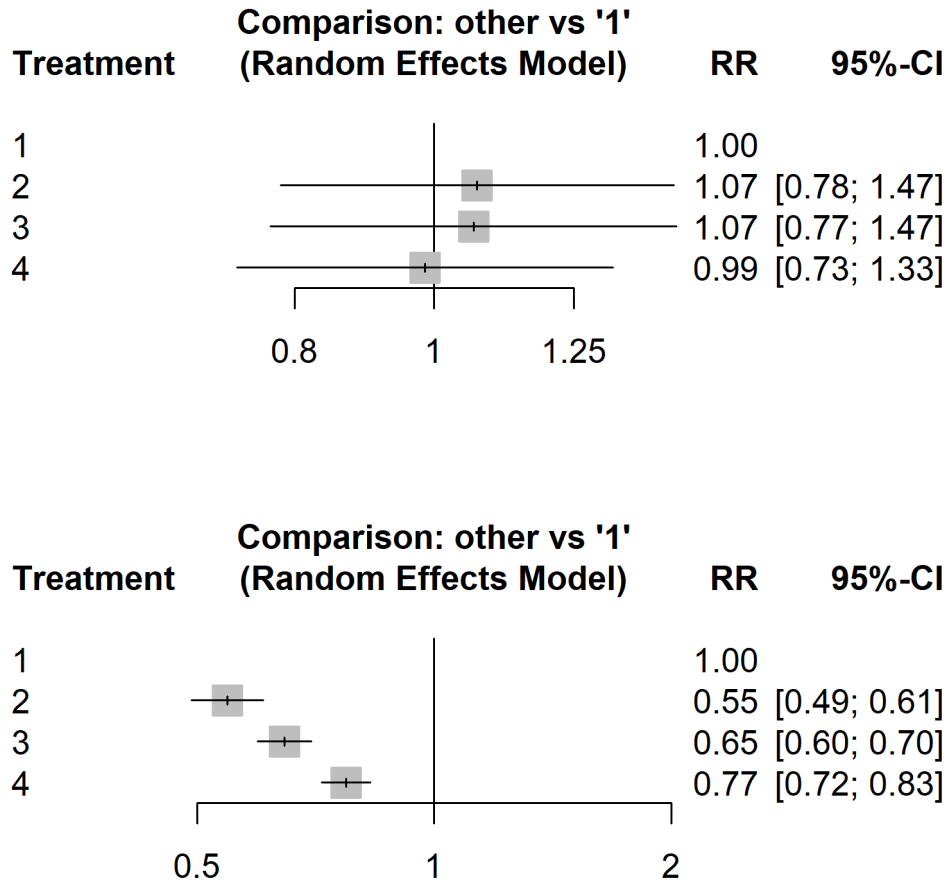

Figure 1: Forest plots showing estimates and 95% CIs for relative effects of network producing the lowest (top) and highest (bottom) POTH in the database of NMAs.

Table 3: Between-study heterogeneity ( $\tau^2$ ),  $I^2$ , and POTH for the two extreme networks in the database.

|                | Lowest POTH Network | Highest POTH Network |
|----------------|---------------------|----------------------|
| $\tau^2$       | 0.00                | 0.00                 |
| $I^2$ (95% CI) | 0% (0-79%)          | 0% (0-37%)           |
| POTH           | 0.096               | 0.999762             |

# 4 What is the Distribution of Precision of Treatment Hierarchies in Networks with No Treatment Differences? A Simulation Study

## 4.1 Set-up

The aim of this simulation study is to understand the distribution of POTH when there are no treatment differences present. We also investigate the impact of network geometry, precision of the data, and heterogeneity on the POTH. We simulated data from a random-effects NMA model where all relative treatment differences are equal to zero, the between-study heterogeneity is equal to  $\tau$ , the observed data in study  $j$  is a mean difference  $y_j$ , and the standard error is given by  $SE(y_j)$ .

$SE(y_j)$  was set to 0.12, 1.10, or 2.07. Between-study heterogeneity  $\tau$  was set to 0 (representing no heterogeneity), 0.12, and 2.07. We investigate three possible network geometries when there are 5 treatments in the network: star, line, and fully connected.

## 4.2 Data Generation

For a given network geometry and settings for  $SE(y_j)$  and  $\tau$ , data was simulated from a random-effects NMA model. The vector of relative effects is set to  $(0, \dots, 0)'$ , so all five treatments are equally effective. Study-specific relative treatment effects are simulated according to

$$\delta_j \sim N(0, \tau^2) \quad (4)$$

for  $j = 1, \dots, M$  where  $M$  is the number of studies in the network. Observed data is simulated according to

$$y_j \sim N(\delta_j, SE(y_j)^2). \quad (5)$$

For each scenario, we simulated 8000 NMA datasets. Each NMA dataset was analysed using a frequentist random-effects NMA model using the R package **netmeta** using the REML method for estimating  $\tau$  [Balduzzi et al., 2023]. The POTH for each simulated NMA dataset was calculated using the **poth** R package.

## 4.3 Results

The mean of POTH observed in the 8000 simulated NMA datasets for each simulation scenario is shown in Figure 2. The mean of POTH for the different settings range from 0.327 to 0.462. For a given level of heterogeneity and network type, as the precision of the data increases, the mean POTH increases. This makes sense, as more precise data will correspond to tighter confidence intervals on the relative effects and therefore higher certainty in the rank probability distributions. In the absence of between-study heterogeneity (where  $\tau = 0$ ), the mean POTH is the smallest for the line network and the largest for the full network. In other words, the more a network relies on indirect evidence, the lower the POTH will be, on average. Finally, we see an increase in the mean POTH as the heterogeneity increases. At first glance this may seem counter-intuitive, however, we speculate that the reason for this trend is that the data are generated assuming no treatment differences. Because of this, as heterogeneity increases, the magnitude of the observed effect sizes in the simulated datasets increases, which can lead to more pronounced differences in P-scores, and thus, higher POTH.

We show the observed distribution of POTH for the combinations of low and high standard error and heterogeneity for all three network types in Figure 3. The fully connected network has the most peaked distributions while the line network has the flattest distributions. Interestingly, in all scenarios, a relatively wide range of POTHs were observed. For all scenarios, the majority of observed POTHs was less than 0.50, but POTHs close to 1 were still observed for a small subset of simulated datasets. This illustrates that POTH can only summarise the certainty in the treatment ranking based on the observed data, and even when no true underlying treatment differences exist, we may still observe data which suggest a clear hierarchy of treatments.

## References

- Sara Balduzzi, Gerta Rücker, Adriani Nikolakopoulou, Theodoros Papakonstantinou, Georgia Salanti, Orestis Efthimiou, and Guido Schwarzer. netmeta: An R Package for Network Meta-Analysis Using Frequentist Methods. *Journal of Statistical Software*, 106:1–40, March 2023. ISSN 1548-7660. doi: 10.18637/jss.v106.i02. URL <https://doi.org/10.18637/jss.v106.i02>.
- Heerajnarain Bulluck, Chun Shing Kwok, Alisdair D. Ryding, and Yoon K. Loke. Safety of short-term dual antiplatelet therapy after drug-eluting stents: An updated meta-analysis with direct and adjusted indirect comparison of randomized control trials. *International Journal of Cardiology*, 181:331–339, February 2015. ISSN 0167-5273. doi: 10.1016/j.ijcard.2014.12.037. URL <https://www.sciencedirect.com/science/article/pii/S0167527314024449>.

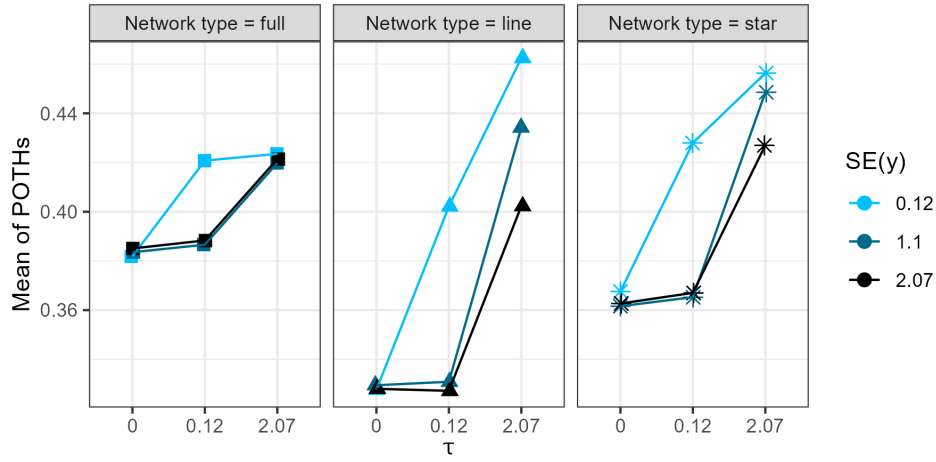

Figure 2: Mean of POTH over the simulated datasets for different combinations of heterogeneity  $\tau$ , network type, and standard error in the data.

Rodrigo Antonini Ribeiro, Patricia Klarmann Ziegelmann, Bruce Bartholow Duncan, Steffan Frosi Stella, José Luiz da Costa Vieira, Luciane Maria Fabian Restelatto, Emílio Hideyuki Moriguchi, and Carisi Anne Polanczyk. Impact of statin dose on major cardiovascular events: A mixed treatment comparison meta-analysis involving more than 175,000 patients. *International Journal of Cardiology*, 166(2):431–439, June 2013. ISSN 0167-5273. doi: 10.1016/j.ijcard.2011.10.128. URL <https://www.sciencedirect.com/science/article/pii/S0167527311020195>.

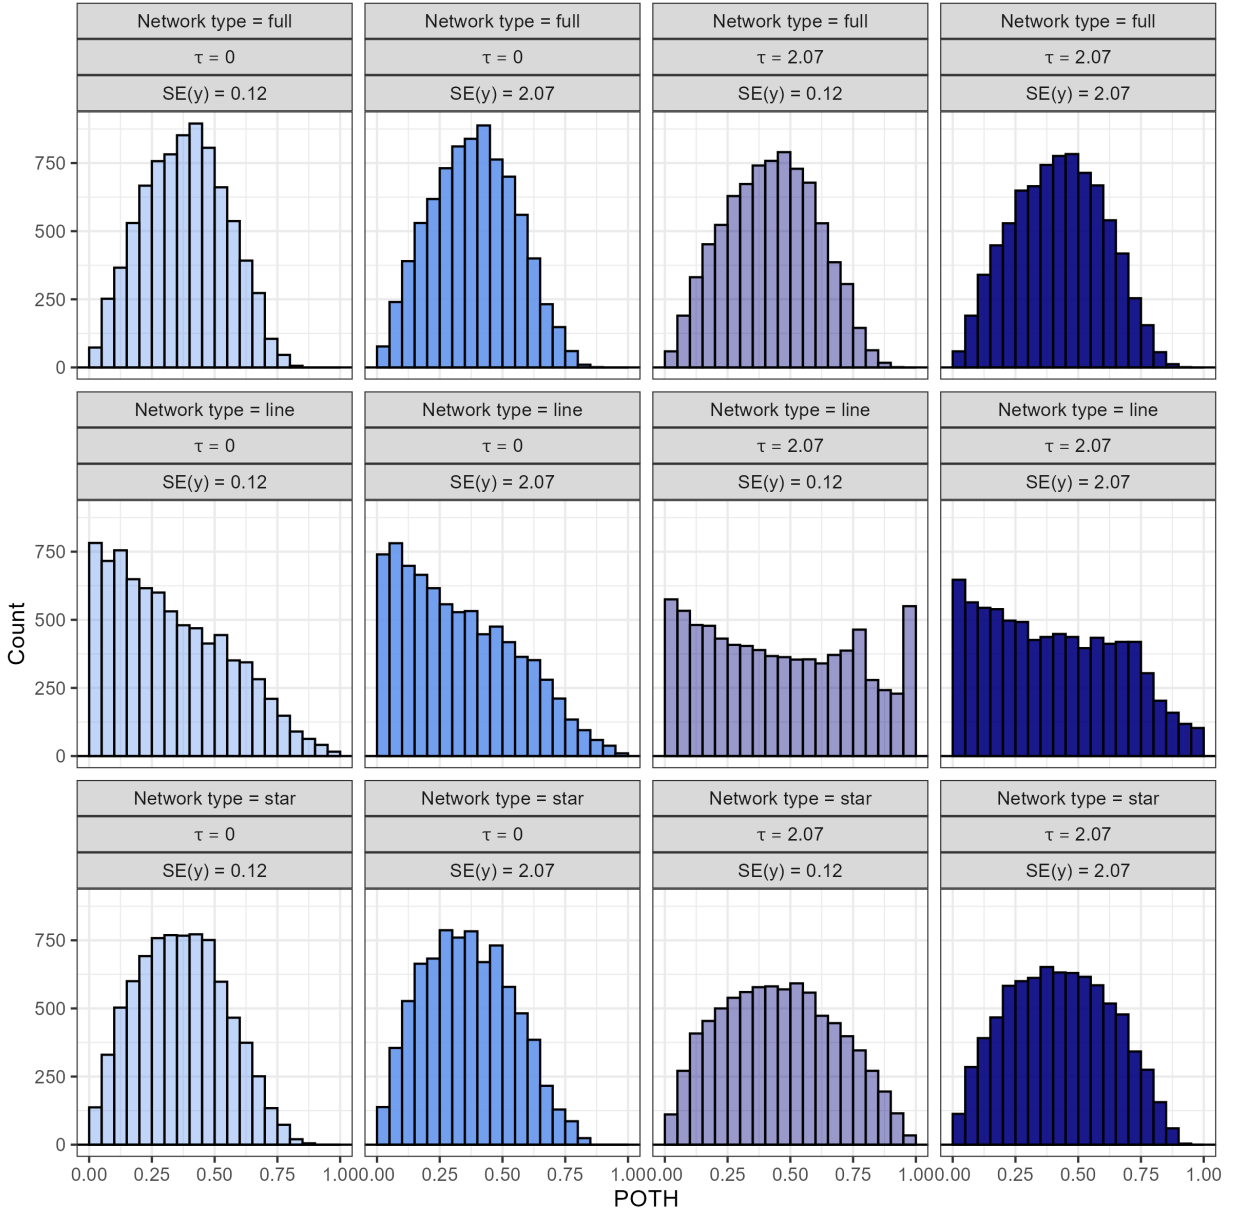

Figure 3: Histograms showing the distribution of POTH observed for different settings in the simulation study.
